# Supplementary material for: Learning Visual-Semantic Subspace Representations
Source: arXiv:2405.16213 source file (2025-04-12)
Supplement: Supplementary file 1 [file appendix_d.tex]

\section{Hilbert space formulation}
\label{sec:app_hilbert}
From the previous formulation, it is clear that the problem becomes intractable as the number of propositions increases, as according to Theorem \ref{theorem:min_nuclear_norm_ell2_squared}, the set of conjunctive clauses in $Y$ will correspond to an orthogonal basis for the representation space. Fortunately, the cost function only depends on the Gram matrix of the embeddings $X^\top X$. In fact,
\begin{equation}
    \left\|\begin{bmatrix}\Yv \\ \Xv\end{bmatrix}\right\|_\ast - \alpha\|\Xv\|_\ast + \beta\|\Xv\|_2^2 = \mathrm{Tr}\left(\left(\Yv^\top \Yv + \Xv^\top \Xv\right)^\frac{1}{2}\right) - \alpha\mathrm{Tr}\left(\left(\Xv^\top \Xv\right)^\frac{1}{2}\right) + \beta \|(\Xv^\top \Xv)\|_2.
\end{equation}
Instead of the encoder mapping each image to a finite-dimensional vector space $\mathbb{R}^d$, we can let the representation space be an infinite dimensional Hilbert space $\mathcal{H}$. Let $k$ be the kernel $k(\xv_i,\xv_j) = \langle\phi(\xv_i), \phi(\xv_j)\rangle$, for some feature map $\phi \in \mathcal{H}$. Replacing $\Xv^\top \Xv$ by $\Kv := [k(\xv_i,\xv_j)]_{ij}$, the kernelized loss becomes
\begin{equation}
     \mathrm{Tr}\left(\left(\Yv^\top \Yv + \Kv\right)^\frac{1}{2}\right) - \alpha\mathrm{Tr}\left(\Kv^\frac{1}{2}\right) + \beta \|\Kv\|_2.
\end{equation}
Provided $k(\xv,\xv)=\langle\phi(\xv),\phi(\xv)\rangle=\|\phi(\xv)\|_2^2=1$ \textit{i.e.}, the features have unit norm in $\mathcal{H}$, the same probabilistic formulation arises. Let $\{\ev_i\}_{i=1}^\infty$ be a countable basis for $\mathcal{H}$ and write $\phi(x)=\sum_{i}^{\infty}a_i e_i$. Then $\|\phi(\xv)\|_2 = \sum_{i}^{\infty} a_i^2 = 1$. Provided different propositions correspond to orthogonal features, then, we can define the posterior probability as $P(\yv_i|\xv):=\langle \phi(\vv),\phi(\xv)\rangle^2 = k(\vv,\xv)^2$.
